# Supplementary material for: Multi-Agent Collaboration for Multilingual Code Instruction Tuning
Source: arXiv:2502.07487 source file (2025-02-11)
Supplement: Supplementary file 1 [file Appendix.tex]

\appendix
